# Supplementary material for: Boosting Learning for LDPC Codes to Improve the Error-Floor Performance
Source: arXiv:2310.07194 source file (2023-10-30)
Supplement: Supplementary file 1 [file Supplementary.pdf]

# 1 Underlying issues addressed in this paper

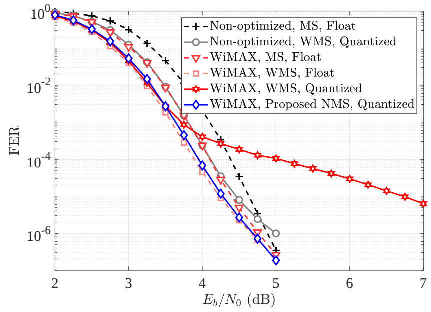


Figure 1: Decoding performance with optimized/non-optimized codes and floating/quanztized decoders.

Generally, LDPC code design assumes the existence of a decoder capable of floating-point operations and optimizes the code to achieve the best waterfall performance. In Fig. 1, it can be observed that the optimized WiMAX LDPC code outperforms the non-optimized regular LDPC code in terms of waterfall performance. Furthermore, to enhance the waterfall performance, the WMS decoder assigns weights to CN messages. As shown in Fig. 1, WMS decoding of the WiMAX LDPC code exhibits the best waterfall performance when floating-point operations are feasible. However, for actual hardware implementation, quantization of decoding messages is essential, but it leads to performance degradation. Particularly, significant performance degradation and early occurrence of error floor can be observed in WMS decoding. By comparing the quantized WMS decoding performances of the non-optimized code and WiMAX LDPC code, we figure out that the degradation due to the quantization occurs more strongly in optimized LDPC codes. Therefore, a method is needed to achieve high performance in both the waterfall and error floor regions at low complexity. This research accomplishes this by employing machine learning techniques to learn the weights. In Fig. 1, the proposed NMS decoder with quantization achieves the floating WMS decoding performance on the both waterfall and error-floor regions.

# 2 Network ensemble v.s. Single large network

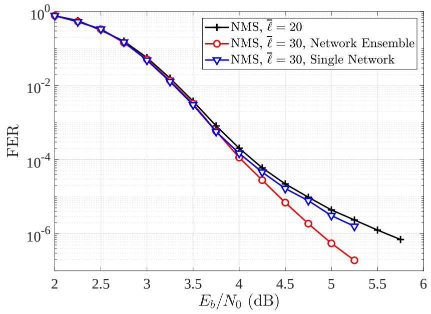


Figure 2: Comparison between the network ensemble and single network.

We compare with the case where, unlike the proposed method, the entire decoding process is not divided into two neural networks but trained with a single neural network by increasing the model size in Fig. 2. The number of iterations is set to 30. For the network ensemble, the proposed boosting learning is conducted by dividing it into a network of iteration 20 and a subsequent network of iteration 10, while the single neural network is trained with 30 iterations at once. Both have the same model size. From the results in Fig. 2, it can be observed that simply increasing the model size does not show a significant effect in removing the error floor. In contrast, the network ensembles with

boosting learning attain decoding diversity and is shown to be more effective in removing the error floor.

## 3 Optimization of parameters of the block-wise training schedule

Table 1: Test FER values of the block-wise training with various $\Delta_1$ and $\Delta_2$

| $\Delta_1 \setminus \Delta_2$ | 0 | 5 | 10 | 15 | 30 |
|---|---|---|---|---|---|
| 1 | 0.376 | 0.144 | 0.123 | 0.122 | 0.150 |
| 5 | 0.193 | 0.134 | **0.112** | 0.127 | 0.137 |
| 10 | 0.142 | 0.142 | 0.13 | 0.128 | 0.13 |
| 30 | 0.179 | | | | |

To optimize the parameters of $\Delta_1$ and $\Delta_2$ in the block-wise training schedule, we calculate the test FER results for uncorrected words with various $\Delta_1$ and $\Delta_2$ values for the training of the post decoder with $\ell_2 = 30$ and summarize them in Table 1. For the case where $\Delta_2 =$ (i.e., without retraining), the performance improves from $\Delta_1 = 1$ to $\Delta_1 = 10$ by training more weights at once to escape from the local minimum. However, if $\Delta_1$ becomes too large, the weights at the front are not sufficiently trained due to the vanishing gradient problem, and accordingly the performance degrades for $\Delta_1 = 30$. In addition, when the number of iterations $\Delta_2$ for retraining is increased for a given $\Delta_1$ value, the same phenomenon occurs, and the performance improves only to a certain extent. From Table 1, the best performance is obtained when $\Delta_1 = 5, \Delta_2 = 10$.

## 4 Discussion on the trained weights

Table 2: Trained weights

| | $\ell$ | Weights | | | | | | | | | |
|---|---|---|---|---|---|---|---|---|---|---|---|
| VW $\overline{w}^{(\ell)}$ | $1 \sim 10$ | 0.74 | 0.98 | 0.96 | 1.10 | 1.20 | 1.15 | 1.22 | 1.19 | 1.17 | 1.09 |
| | $11 \sim 20$ | 1.15 | 1.09 | 1.07 | 1.04 | 1.05 | 1.07 | 1.00 | 0.98 | 0.90 | 0.81 |
| | $21 \sim 30$ | 1.14 | 0.97 | 0.93 | 0.69 | 0.66 | 0.58 | 0.57 | 0.51 | 0.49 | 0.45 |
| | $31 \sim 40$ | 0.48 | 0.41 | 0.37 | 0.38 | 0.38 | 0.39 | 0.32 | 0.33 | 0.32 | 0.34 |
| | $41 \sim 50$ | 0.39 | 0.37 | 0.31 | 0.31 | 0.34 | 0.45 | 0.39 | 0.37 | 0.42 | 0.42 |
| CW $w^{(\ell)}$ | $1 \sim 10$ | 0.74 | 0.71 | 0.66 | 0.69 | 0.67 | 0.70 | 0.75 | 0.71 | 0.73 | 0.76 |
| | $11 \sim 20$ | 0.73 | 0.70 | 0.77 | 0.79 | 0.84 | 0.84 | 0.86 | 0.82 | 0.81 | 0.97 |
| | $21 \sim 30$ | 0.19 | 0.30 | 0.54 | 0.58 | 0.62 | 0.59 | 0.73 | 0.73 | 0.74 | 0.78 |
| | $31 \sim 40$ | 0.72 | 0.78 | 0.79 | 0.81 | 0.88 | 0.82 | 0.88 | 0.85 | 0.97 | 0.79 |
| | $41 \sim 50$ | 0.81 | 0.82 | 0.85 | 0.91 | 1.19 | 0.86 | 0.96 | 1.10 | 1.18 | 1.62 |
| UCW $\hat{w}^{(\ell)}$ | $1 \sim 10$ | 0.74 | 0.71 | 0.66 | 0.69 | 0.67 | 0.70 | 0.75 | 0.71 | 0.73 | 0.76 |
| | $11 \sim 20$ | 0.73 | 0.70 | 0.77 | 0.79 | 0.84 | 0.84 | 0.86 | 0.82 | 0.81 | 0.97 |
| | $21 \sim 30$ | 0.58 | 0.80 | 0.83 | 0.73 | 0.81 | 0.86 | 0.72 | 0.78 | 0.73 | 0.73 |
| | $31 \sim 40$ | 0.59 | 0.71 | 0.64 | 0.67 | 0.67 | 0.72 | 0.65 | 0.65 | 0.66 | 0.70 |
| | $41 \sim 50$ | 0.77 | 0.70 | 0.72 | 0.81 | 0.92 | 0.58 | 0.71 | 0.76 | 0.87 | 1.57 |

Table 2 shows the trained weights using the proposed trainig methods. Due to the use of the spatial weight sharing technique, only three types of weights, variable weight (VW) $\overline{w}^{(\ell)}$, check node weight (CW) $w^{(\ell)}$, and unsatisfied check node weight (UCW) $\hat{w}^{(\ell)}$, exist for each iteration. Therefore, the variation of weights with respect to iterations can be represented in two dimensions, as shown in Fig. 3(a), enabling analysis of the trained results. If the weight sharing technique is not used, there would be $(N + E)$ weights for each iteration, making it impossible to analyze them in a 2D graph. Fig. 3(a) shows that the weights during the base decoding stage are similar to the weights of conventional WMS decoding, where the CW and VW are $0.75$ and $1$, respectively. Therefore, the performance of WMS decoding and NMS decoding turns out to be similar. In other words, the base NMS decoder provides little gain in the waterfall region.

On the other hand, for the post decoding stage, the weights undergo significant changes. At iteration 21, the VW increases while the CW decreases substantially. This means that the channel LLR values are given more weight when performing the sum operation at each VN, while the messages coming

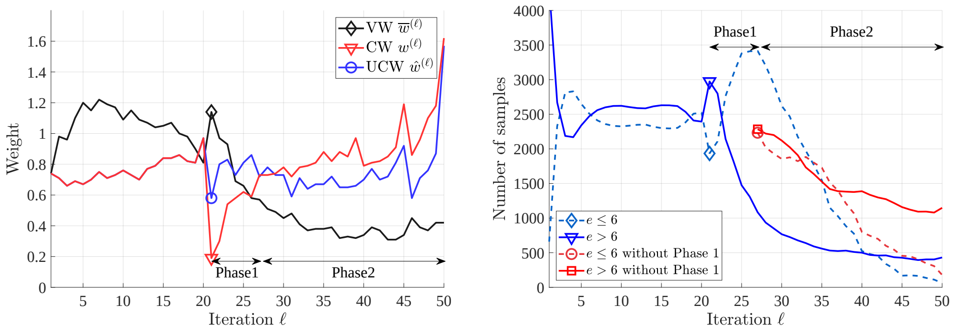


(a) (b)

Figure 3: Evolution of the weights and the number of samples as a function of iteration.

from CNs are attenuated. As a result, the decoding process regresses to the initial decoding state (with a high error rate), leading to an increase in the number of samples having more than 6 errors (denoted by $e > 6$), as shown in Fig. 3(b), and a decrease in the number of samples with $e \leq 6$. This regression to the initial state aims to break free from trapped error patterns. From iteration 22 onward, the CW gradually increases, the VW decreases, and the number of $e \leq 6$ samples starts to increase again. After iteration 27, the CW and VW show less significant variations, which we refer to as Phase 2, while Iterations 21 to 26 are referred to as Phase 1. At iteration 20, the number of samples with $e \leq 6$ and $e > 6$ are similar, but through Phase 1, samples with $e > 6$ transformed into samples with $e \leq 6$. Consequently, by the end of Phase 1, there are more samples with $e \leq 6$ than samples with $e > 6$. The small-sized error samples are gradually decreased in Phase 2.

The result without Phase 1 is shown in Fig. 3(b). Without Phase 1, the process of transforming into small-sized error samples is omitted. Consequently, the decoding proceeds in a situation where the number of samples with $e \leq 6$ and $e > 6$ is similar. Although the $e \leq 6$ samples are mostly corrected through Phase 2, the $e > 6$ samples remain in significant numbers as they are initially abundant. This indicates the need for the pre-processing of Phase 1.
